# Supplementary material for: Strong enhancement of g-factor in PbTe-Pb hybrid nanowires
Source: arXiv:2502.07477 source file (2026-04-02)
Supplement: Supplementary file 1 [file PbTe_ZBP_SM.pdf]

# Supplemental Material for “Robust zero modes in PbTe-Pb hybrid nanowires”

Shan Zhang,<sup>1,\*</sup> Wenyu Song,<sup>1,\*</sup> Zonglin Li,<sup>1,\*</sup> Zehao Yu,<sup>1,\*</sup> Ruidong Li,<sup>1</sup> Yuhao Wang,<sup>1</sup> Zeyu Yan,<sup>1</sup> Jiaye Xu,<sup>1</sup> Zhaoyu Wang,<sup>1</sup> Yichun Gao,<sup>1</sup> Shuai Yang,<sup>1</sup> Lining Yang,<sup>1</sup> Xiao Feng,<sup>1,2,3,4</sup> Tiantian Wang,<sup>2,4</sup> Yunyi Zang,<sup>2,4</sup> Lin Li,<sup>2</sup> Runan Shang,<sup>2,4</sup> Qi-Kun Xue,<sup>1,2,3,4,5</sup> Ke He,<sup>1,2,3,4,†</sup> and Hao Zhang<sup>1,2,3,‡</sup>

<sup>1</sup>State Key Laboratory of Low Dimensional Quantum Physics,

Department of Physics, Tsinghua University, Beijing 100084, China

<sup>2</sup>Beijing Academy of Quantum Information Sciences, Beijing 100193, China

<sup>3</sup>Frontier Science Center for Quantum Information, Beijing 100084, China

<sup>4</sup>Hefei National Laboratory, Hefei 230088, China

<sup>5</sup>Southern University of Science and Technology, Shenzhen 518055, China

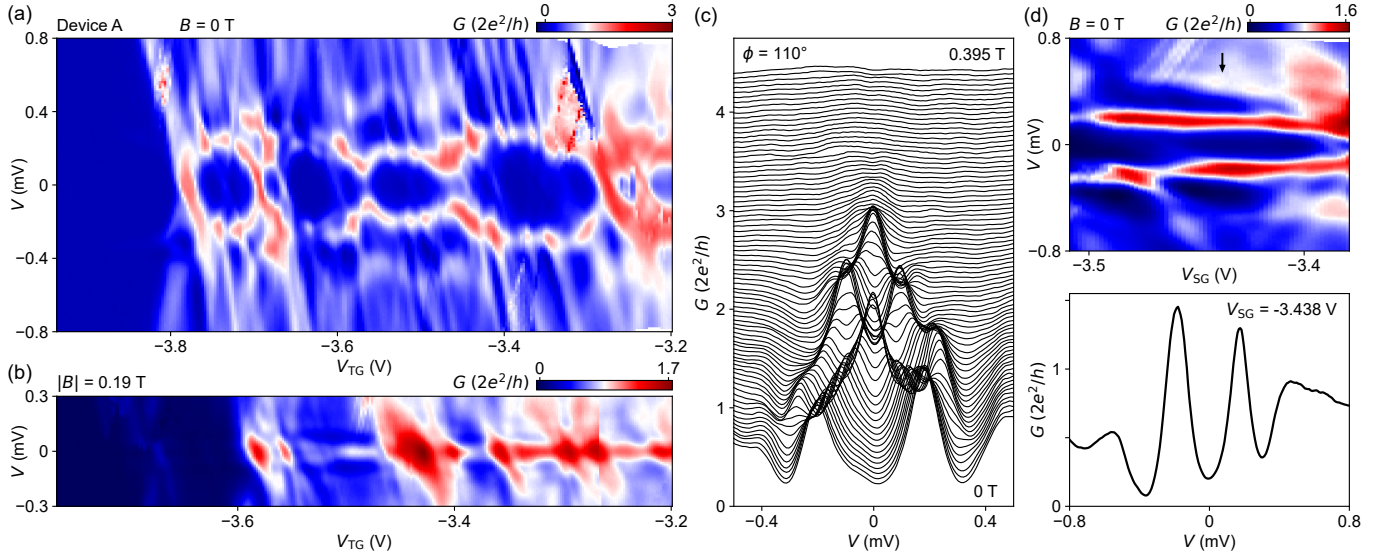

FIG. S1. (a) Tunneling spectroscopy of device A at zero field. The SG was scanned together with the TG, i.e.  $V_{SG} = V_{TG}$ . ABSs due to formation of unintentional quantum dots can be revealed. No robust ZBPs are observed at zero field. (b) Gate scan at 0.19 T over a larger range compared to Fig. 1(e).  $\theta = 90^\circ$ ,  $\phi = 110^\circ$ . A robust ZBP can be revealed. (c) Waterfall plot of Fig. 1(b) with a vertical offset of  $0.05 \times 2e^2/h$ . (d)  $V_{SG}$  scan at zero field.  $V_{TG} = -3.764$  V. The lower panel shows a vertical line cut (see the black arrow in the upper panel) of the two subgap peaks. The gap size is near 0.49 meV.

\* equal contribution

† kehe@tsinghua.edu.cn

‡ hzquantum@mail.tsinghua.edu.cn

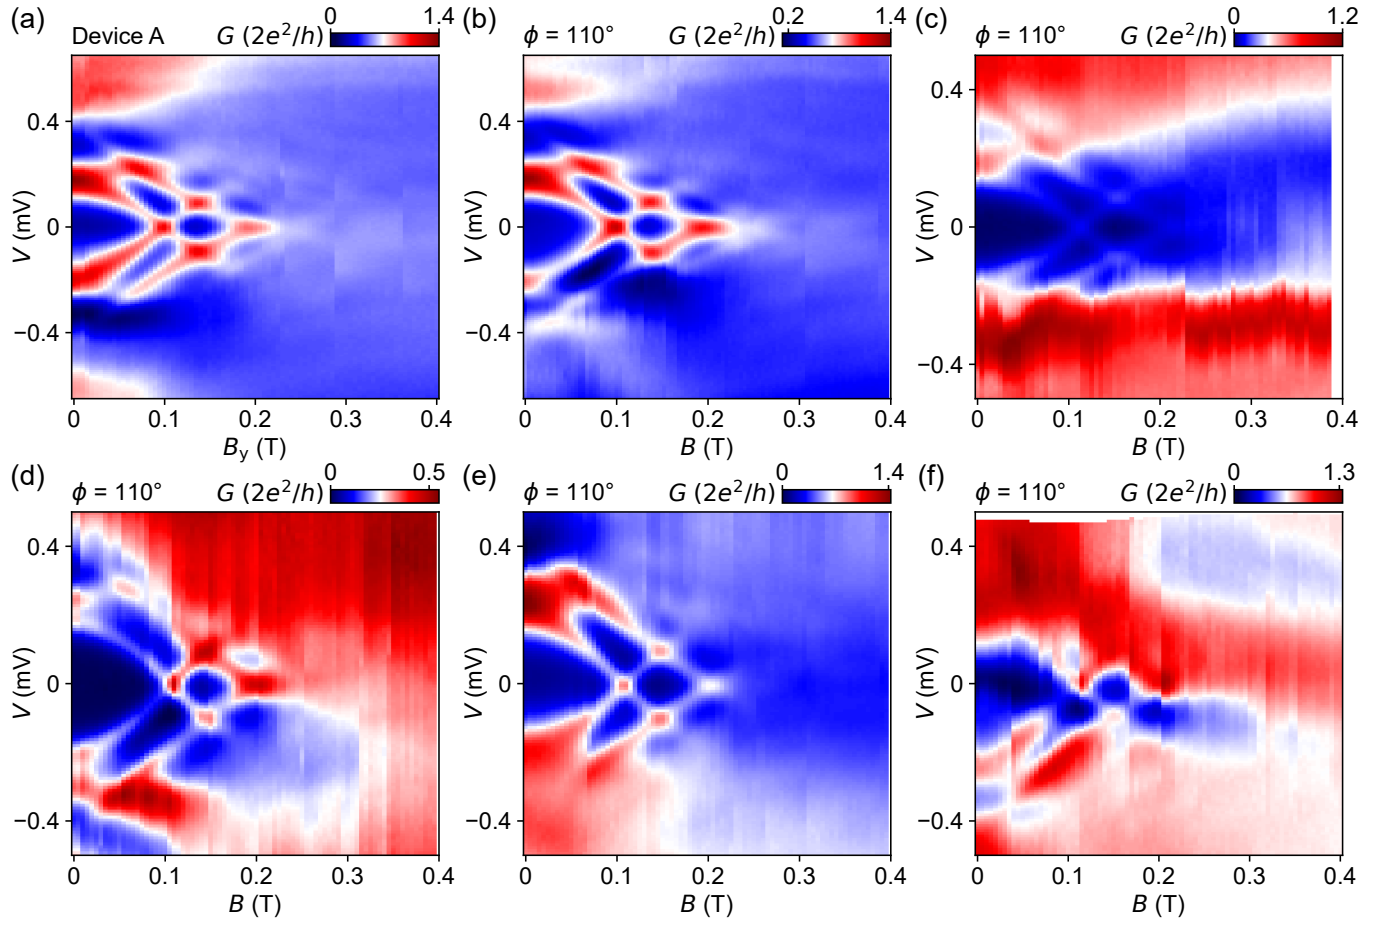

FIG. S2. Additional  $B$  scans at various gate voltages.  $V_{TG} = -3.714$  V,  $-3.714$  V,  $-3.9$  V,  $-3.814$  V,  $-3.814$  V,  $-3.814$  V, while  $V_{SG} = -3.456$  V,  $-3.444$  V,  $-4.151$  V,  $-3.82$  V,  $-3.93$  V,  $-4.026$  V, for panels (a-f).  $\theta = 90^\circ$ ,  $\phi = 110^\circ$  for (b-f), while for (a)  $B$  is aligned with the  $y$  axis. At some gate voltages, the  $B$  scan reveals no robust ZBPs.

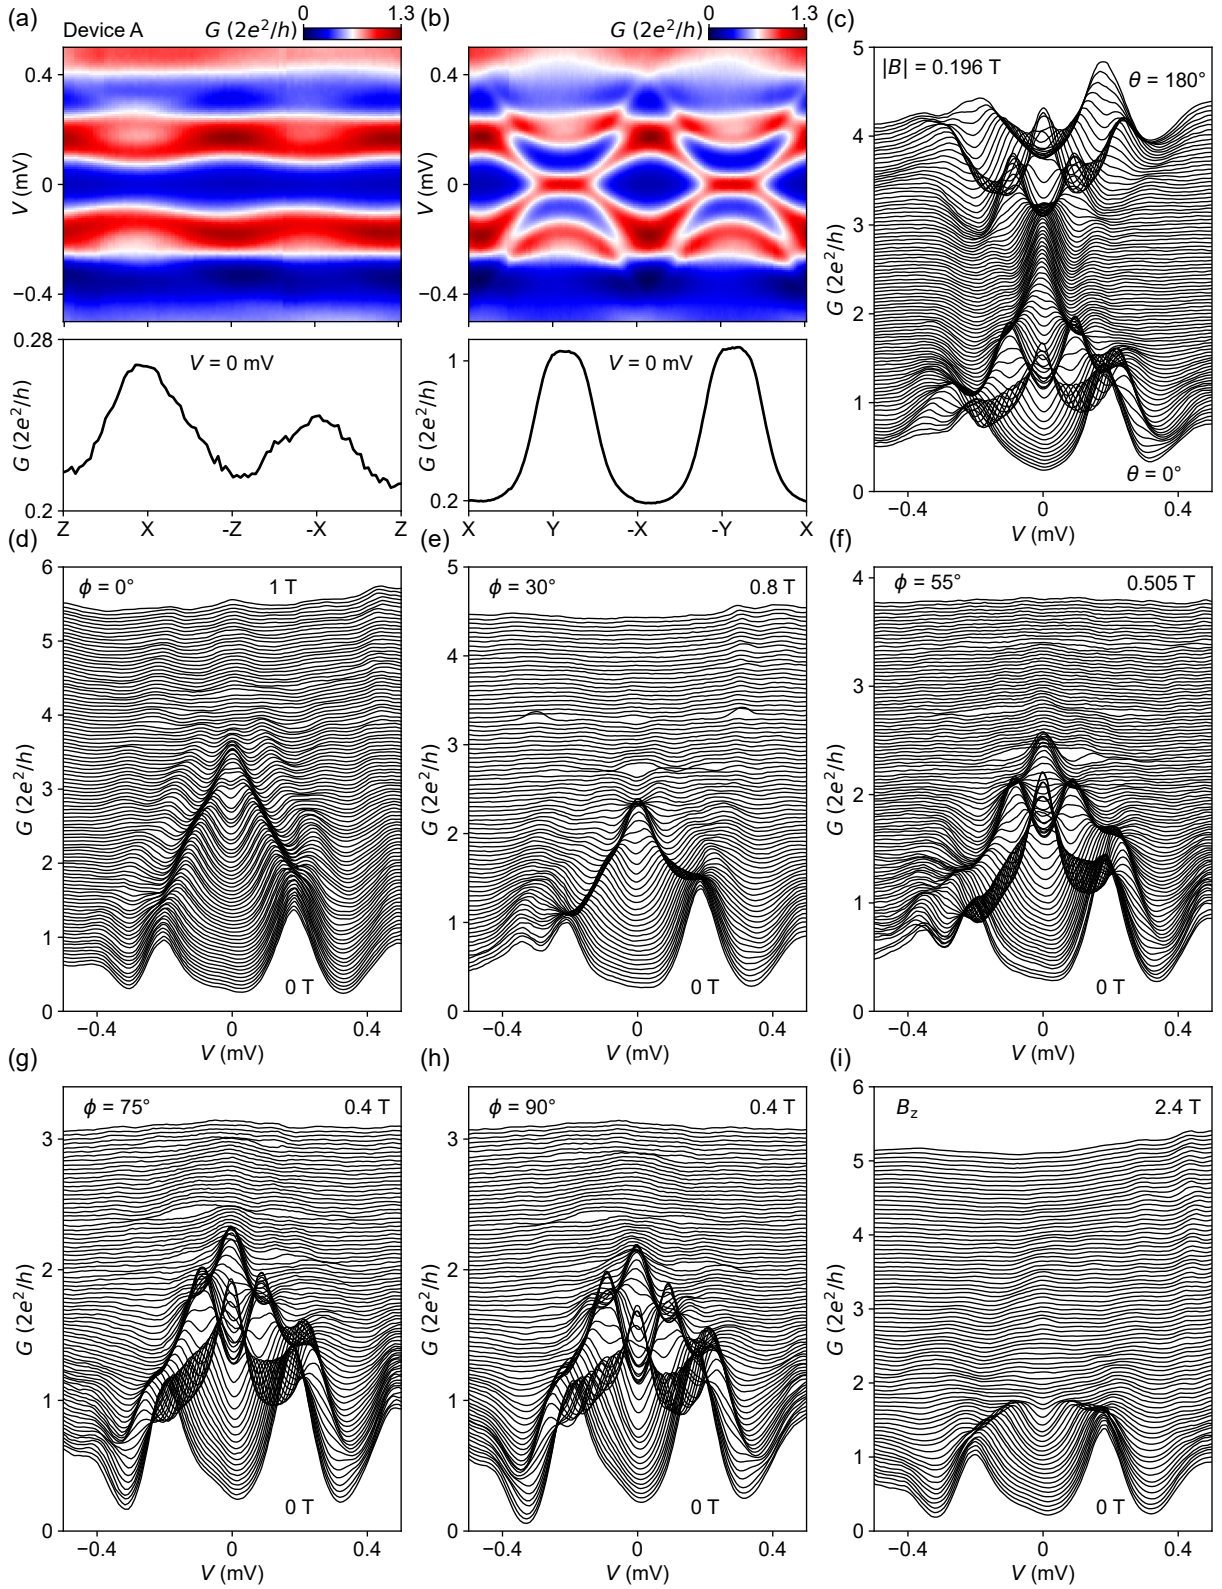

FIG. S3. (a)  $B$  rotation in the  $xz$  plane for  $|B|$  fixed at 0.196 T. Gate settings are the same with that in Figs. 2(a-b). Lower panel, zero-bias line cut. (b)  $B$  rotation in the  $xy$  plane for  $|B|$  fixed at 0.1 T. This ZBP corresponds to the non-robust one in Fig. 1(b). (c) Waterfall plot of Fig. 2(c) with a vertical offset of  $0.04 \times 2e^2/h$ . (d-i) Waterfall plots of Figs. 2(e-f). The vertical offsets (in units of  $2e^2/h$ ) are 0.05, 0.05, 0.0325, 0.0325, 0.0325, and 0.06, respectively.

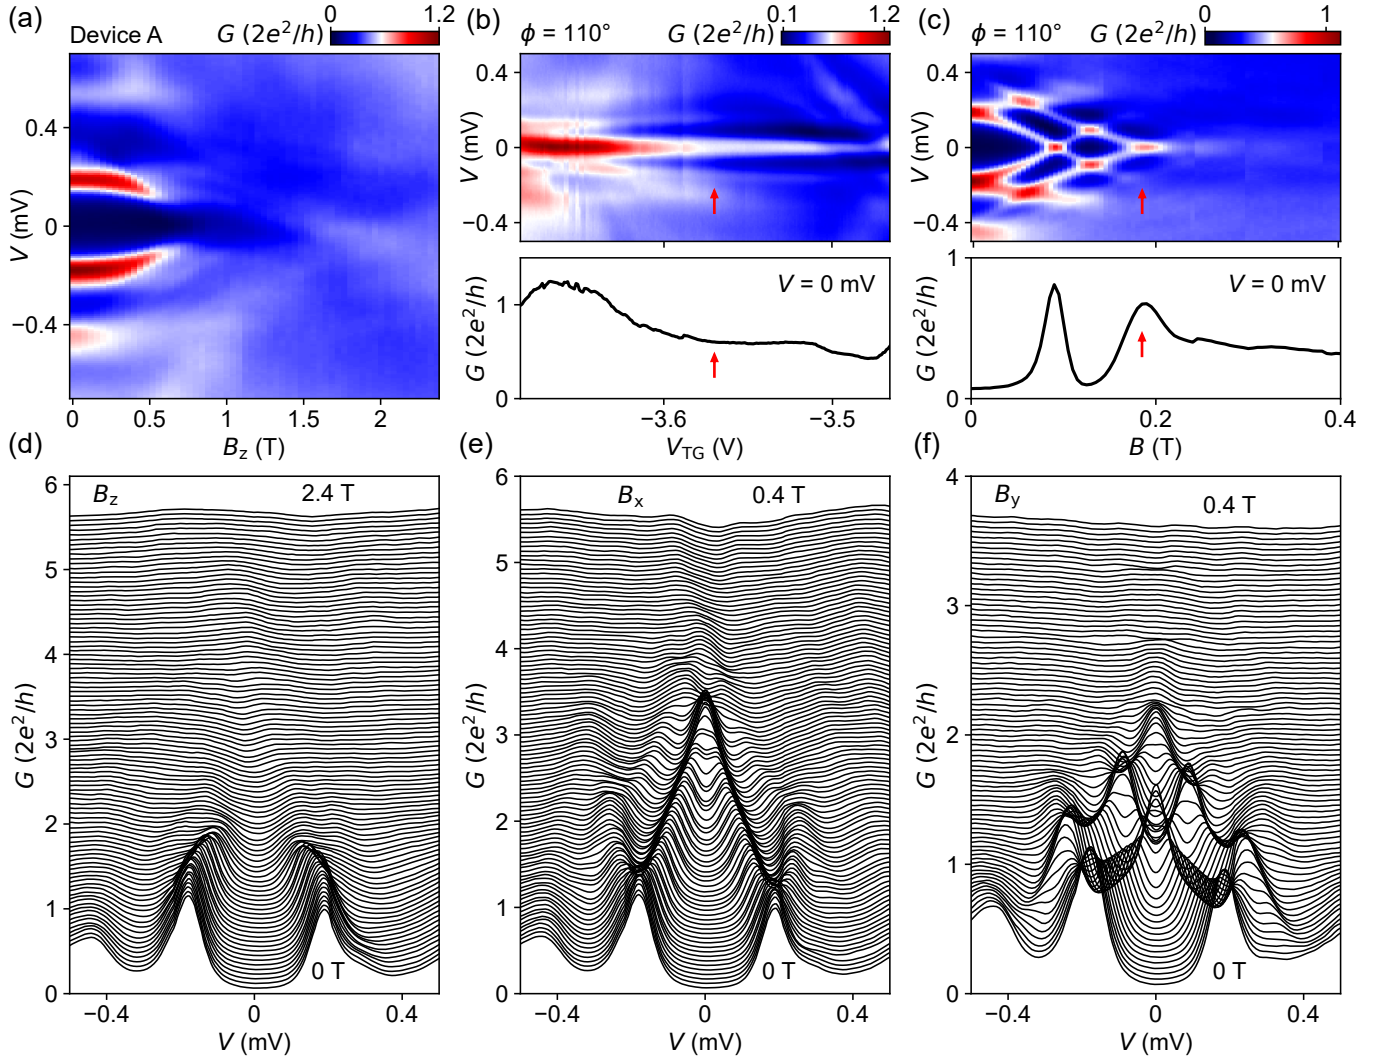

FIG. S4. (a)  $B_z$  scan of the ZBP in Figs. 3(a-b). No ZBP is revealed for  $B$  along this direction due to a small effective  $g$ -factor. (b)  $V_{TG}$  scan of the ZBP in Fig. 3. The lower panel shows the zero-bias line cut. The region labeled by the red arrow marks a "plateau-like" feature in  $V_{TG}$  scan. It is in fact not a true plateau, as the corresponding  $B$  scan shown in (c) does not reveal a plateau near this region (the red arrow). (c) Replot of Fig. 3(f) with zero-bias line cut shown in the lower panel. (d-f) Waterfall plots of panel (a), Fig. 3(a), and Fig. 3(b), respectively. The vertical offsets (in units of  $2e^2/h$ ) are 0.055, 0.02, and 0.041, respectively.

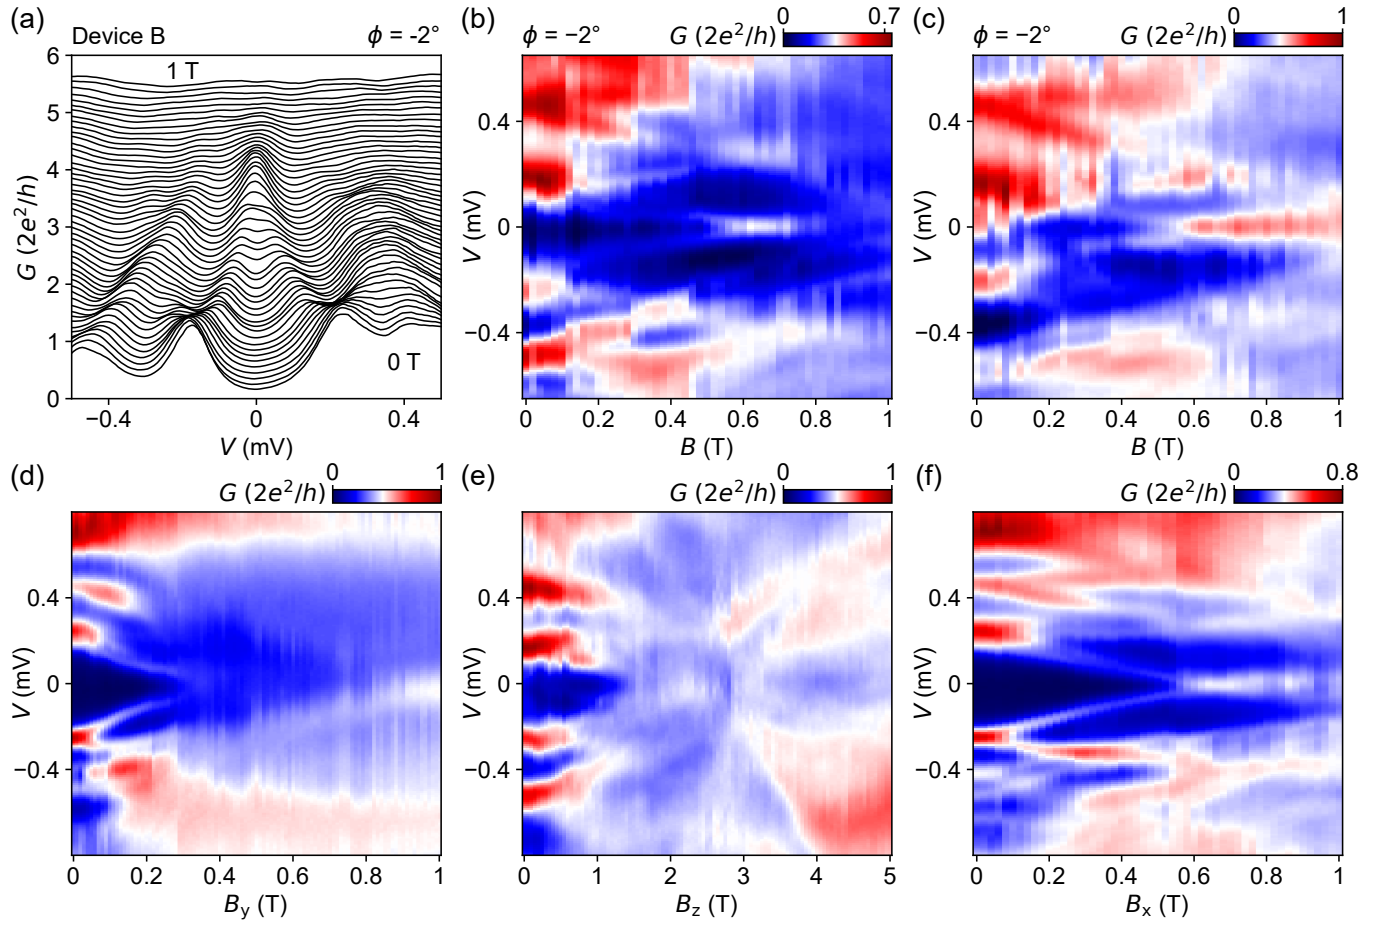

FIG. S5. (a) Waterfall plot of Fig. 4(f) with a vertical offset of  $0.1 \times 2e^2/h$ . (b-c) Two additional  $B$  scans in device B.  $\theta = 90^\circ$ ,  $\phi = -2^\circ$ ,  $V_{TG} = -2$  V.  $V_{SG} = -7.54$  V and  $-7.35$  V, respectively. (d-f)  $B$  scans along three axes.  $V_{SG} = -7$  V.  $V_{TG} = -1.77$  V,  $-1.77$  V, and  $-1.94$  V, respectively.

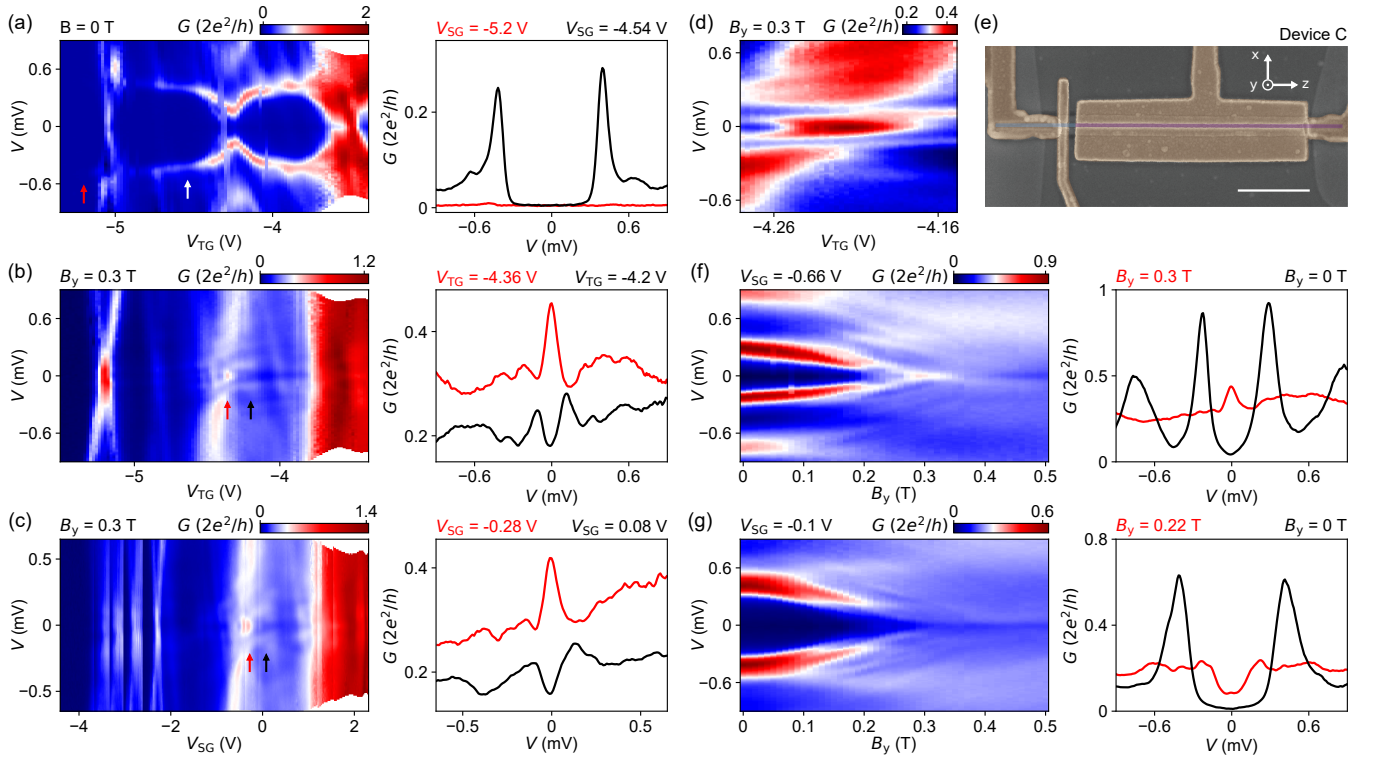

FIG. S6. An example of non-robust ZBP in device C. (a) Zero-field tunneling spectroscopy.  $V_{SG} = 0$  V. Right panel, vertical line cuts at -5.2 V and -4.54 V (see the arrows in the left panel). (b-c)  $V_{TG}$  and  $V_{SG}$  scans at  $B_y = 0.3$  T.  $V_{SG} = 0$  V for (b) and  $V_{TG} = -4.23$  V for (c). A ZBP is revealed (the red arrow), see the red line cuts in the right panels. This ZBP is non-robust and caused by a dot state crossing zero energy. The black curves correspond to the line cuts marked by the black arrows. (d) Fine measurement near this ZBP.  $V_{SG} = -0.66$  V. The “tilted red region” indicates the dot state, which can be fine-tuned to zero by  $V_{TG}$ , causing a ZBP. (e) False-colored SEM of device C. Scale bar, 1  $\mu m$ . (f)  $B_y$  scan of this ZBP.  $V_{SG} = -0.66$  V.  $V_{TG} = -4.216$  V. The ZBP is also non-robust in  $B$  scan and quickly splits with increasing  $B$ . Right panel, line cuts at 0 T and 0.3 T. (g)  $B_y$  scan at a different gate setting, revealing no ZBPs.  $V_{SG} = -0.1$  V.  $V_{TG} = -4.216$  V.
